# Supplementary material for: Designing Thermoplasmonic Properties of Metallic Metasurfaces
Source: arXiv:1804.01111 ancillary file (2018-04-03)
Supplement: Supplementary file 1 [file sup-jop-cg-pw.pdf]

# Designing Thermoplasmonic Properties of Metallic Metasurfaces: Supplemental Informations

Christian Girard, Peter R. Wiecha, Aurélien Cuche, and Erik Dujardin

CEMES CNRS UPR 8011 and Université de Toulouse, 29 rue Jeanne Marvig, BP 94347, 31055 Toulouse cedex 4, France.

e-mail: girard@cemes.fr

## 1 Relationship between temperature distribution and heat flow induced in two-dimensional plasmonic systems

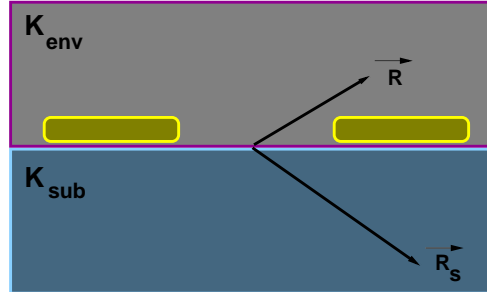

Figure 1: (color online) Side view of a system consisting of metal nanostructures (in yellow color) immersed in water and supported by a glass substrate. The heat flow expected around the metal nanostructures can be derived from the temperature distributions lying in the two half spaces.

In the immediate vicinity of the metal patterns (cf. figure (1)), the temperature distribution must be calculated taking into account the effect of the substrate. As described in refs. [1] and [2], this coupling thermal effect can be treated using the image method. In first medium (water), that leads to:

$$\Delta T(\mathbf{R}) = \frac{1}{4\pi\kappa_{env}} \sum_{p=1}^N \sum_{j=1}^{n_p} \mathcal{Q}(\mathbf{r}_{p,j}) \left\{ \frac{1}{|\mathbf{R} - \mathbf{r}_{p,j}|} + \frac{\kappa_{sub} - \kappa_{env}}{\kappa_{sub} + \kappa_{env}} \frac{1}{|\mathbf{R} - \mathbf{r}'_{p,j}|} \right\}, \quad (1)$$

where  $\kappa_{sub}$  and  $\kappa_{env}$  represent the thermal conductivity of the two half spaces, and  $\mathbf{r}'_{p,j} = (x_{p,j}, y_{p,j}, -z_{p,j})$  is the image position of  $\mathbf{r}_{p,j}$  in the metal. In the glass substrate, we have a similar relation:

$$\Delta T(\mathbf{R}_{sub}) = \frac{1}{4\pi\kappa_{sub}} \sum_{p=1}^N \sum_{j=1}^{n_p} \mathcal{Q}(\mathbf{r}_{p,j}) \left\{ \frac{2\kappa_{sub}}{\kappa_{sub} + \kappa_{env}} \frac{1}{|\mathbf{R}_{sub} - \mathbf{r}_{p,j}|} \right\}. \quad (2)$$

In equation (1), the second term accounts for the thermal reflection generated by the surface. In the first half space (water), we note that this contribution rapidly vanishes when increasing the observation distance leading to the relation (23) introduced in the main text. At shorter distance from the metal pattern the complete relation (1) should be chosen for all temperature computations. From these two relations, (1) and (2), one can

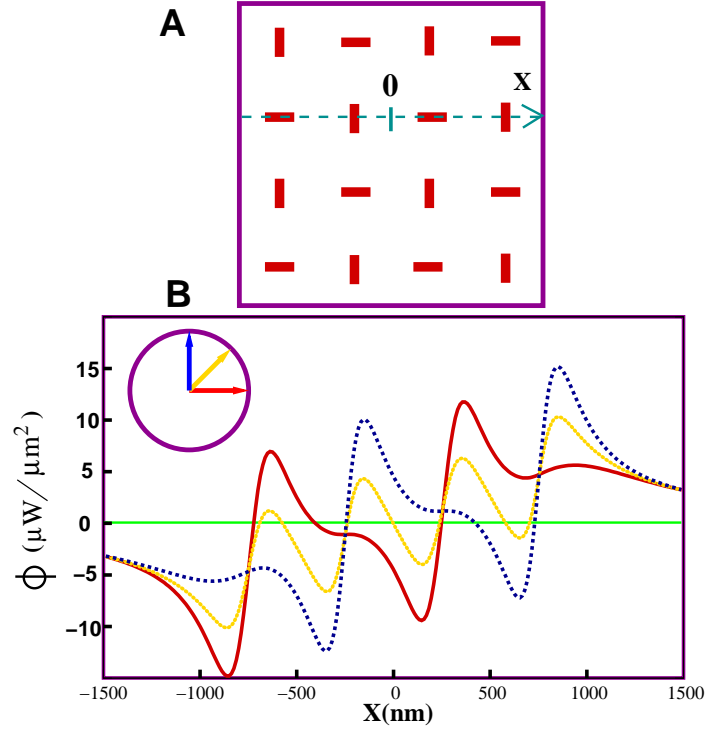

Figure 2: (color online) Top view of the thermoplasmonic metasurface described in figure (5) of the main text: the horizontal dashed line represents the scanline used for the heat flow computation. (B) Example of heat flows computed above the metasurface at a distance of 100nm from the gold nanorods. As in the previous calculations presented in the main text, the surface is illuminated in normal incidence by a plane wave tunable in polarization. The three color plots corresponds to the polarization direction indicated by the red, yellow, and blue arrows in the circular inset. These curves demonstrate the lateral control of the heat flow along the ( $OX$ ) axis by turning the incident polarization from  $0^\circ$  to  $90^\circ$ .

accurately calculate the heat generated by the plasmonic structures and flowing in their

immediate vicinity, both in the water and in the glass. This effect is usually described by a field of vectors  $\Phi(\mathbf{R})$  defined by:

$$\Phi(\mathbf{R}) = -\kappa_{env} \nabla_{\mathbf{r}=\mathbf{R}}[\Delta T(\mathbf{r})] , \quad (3)$$

inside the water, and:

$$\Phi(\mathbf{R}_s) = -\kappa_{sub} \nabla_{\mathbf{r}=\mathbf{R}_s}[\Delta T(\mathbf{r})] , \quad (4)$$

in the glass substrate. A first example of application of equation (3) is given in figure (2).

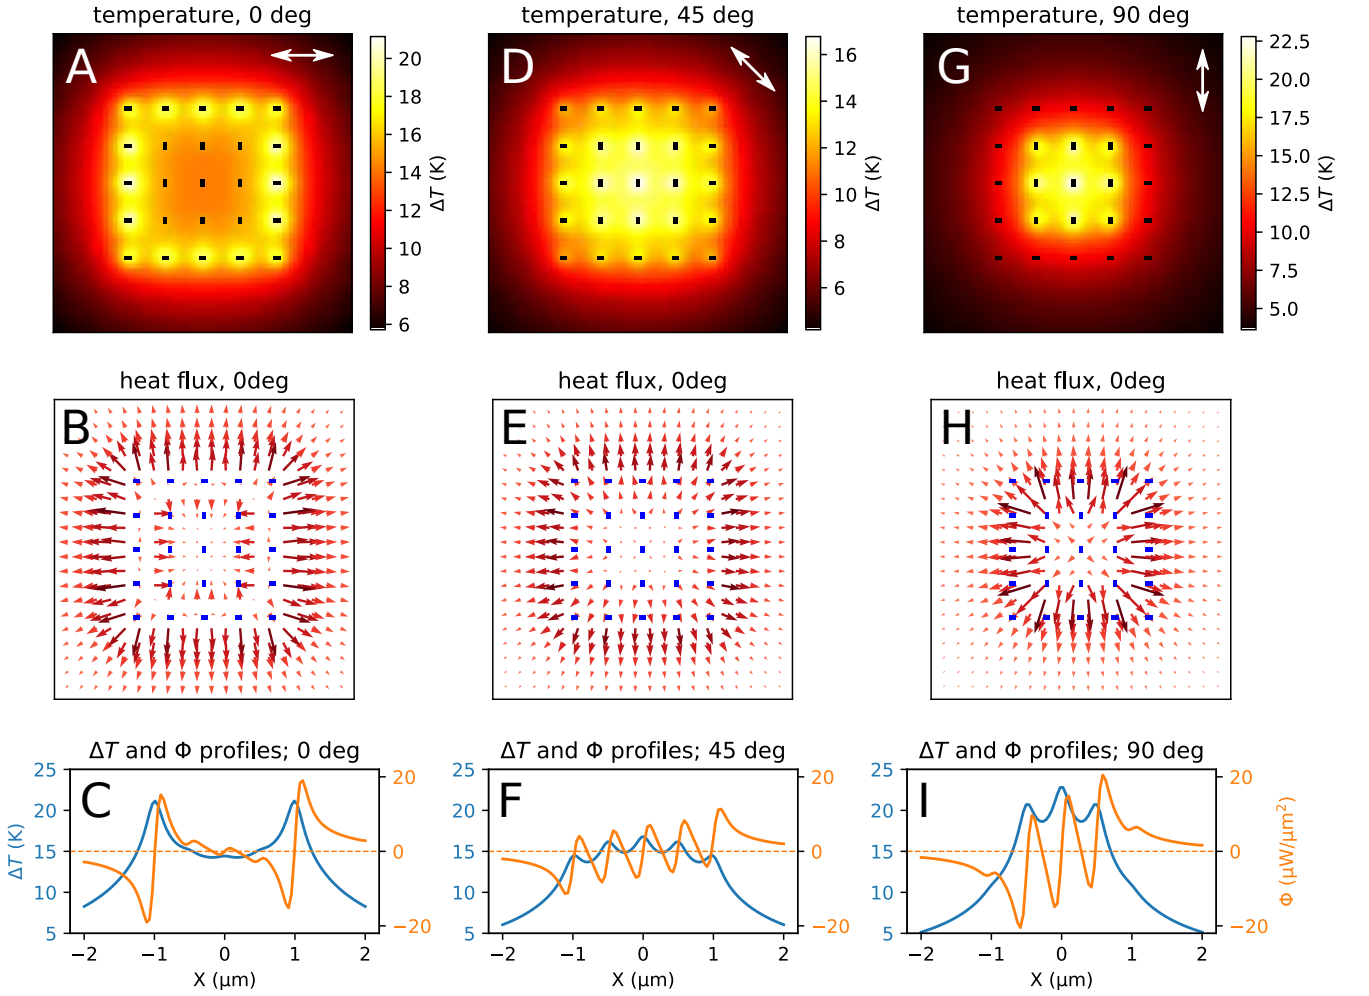

Figure 3: (color online) Plasmonic metasurface for the control of the heat flow. Incident plane wave with  $\lambda_0 = 800$  nm and a linear polarization angle of (A-C)  $0^\circ$ , (D-F)  $45^\circ$ , and (G-I)  $90^\circ$ . (A,D,G) show mappings of the temperature rise  $\Delta T$ , 100 nm above the gold rod top surfaces. (B,E,H) show the heat flow  $\Phi(\mathbf{R})$  in the same plane. (C,F,I) show profiles of  $\Delta T$  and  $\Phi(\mathbf{R})$  along (OX), hence through the center of the metasurface. All mappings show areas of  $4 \times 4 \mu m^2$ .

## 2 Metasurfaces for heat flow control

A further example of heat flow calculation via equation (3) is given in figure 3. In this second example, we show a small metasurface of  $(5 \times 5)$  elements, which can be used to redirect the two-dimensional heat-flow as function of the polarization. The metasurface consists of gold-rods of size  $(30 \times 75 \times 30) \text{ nm}^3$ , lying on a glass substrate in water (Glass:  $n = 1.5$ ,  $\kappa = 0.8 \text{ Wm}^{-1}\text{K}^{-1}$ ; Water: Glass:  $n = 1.33$ ,  $\kappa = 0.6 \text{ Wm}^{-1}\text{K}^{-1}$ ). The outer rods of the metasurface are aligned along  $(OX)$  while the  $(9 \times 9)$  rods in its interior are oriented along  $(OY)$ . For an illumination by an  $(OX)$ -polarized plane wave (in the example,  $\lambda_0 = 800 \text{ nm}$ ), mainly the outer “layer” of rods is heating the environment, leading to an inwards directed heat-flux above the center of the metasurface (Fig. 3A-C). If the polarization is rotated, for angles higher than  $45^\circ$ , the “inner” rods are contributing more significantly to the heat generation, leading to a purely outwards directed heat flow (Fig. 3D-I).

## References

- [1] G. Baffou, R. Quidant, and Ch. Girard, *Phys. Rev. B* **82**, 165424–11 (2010).
- [2] G. Baffou and R. Quidant, *Laser and Photonics Reviews*, **7**, 171 (2013).
